# Supplementary material for: Evaluating Dialect Robustness of Language Models via Conversation Understanding
Source: arXiv:2405.05688 source file (2024-12-11)
Supplement: Supplementary file 1 [file supplementary-material.tex]

% \documentclass[a4paper]{article}

% %% Language and font encodings
% \usepackage{times}  % DO NOT CHANGE THIS
% \usepackage{helvet}  % DO NOT CHANGE THIS
% \usepackage{courier}  % DO NOT CHANGE THIS
% \usepackage[hyphens]{url}  % DO NOT CHANGE THIS
% \usepackage{graphicx} % DO NOT CHANGE THIS
% \urlstyle{rm} % DO NOT CHANGE THIS
% \def\UrlFont{\rm}  % DO NOT CHANGE THIS
% \usepackage{natbib}  % DO NOT CHANGE THIS AND DO NOT ADD ANY OPTIONS TO IT
% \usepackage{caption} % DO NOT CHANGE THIS AND DO NOT ADD ANY OPTIONS TO IT
% \frenchspacing  % DO NOT CHANGE THIS
% \setlength{\pdfpagewidth}{8.5in} % DO NOT CHANGE THIS
% \setlength{\pdfpageheight}{11in} % DO NOT CHANGE THIS
% %
% % These are recommended to typeset algorithms but not required. See the subsubsection on algorithms. Remove them if you don't have algorithms in your paper.
% \usepackage{algorithm}
% \usepackage{algorithmic}

% %
% % These are are recommended to typeset listings but not required. See the subsubsection on listing. Remove this block if you don't have listings in your paper.
% \usepackage{newfloat}
% \usepackage{listings}
% \DeclareCaptionStyle{ruled}{labelfont=normalfont,labelsep=colon,strut=off} % DO NOT CHANGE THIS
% \lstset{%
% 	basicstyle={\footnotesize\ttfamily},% footnotesize acceptable for monospace
% 	numbers=left,numberstyle=\footnotesize,xleftmargin=2em,% show line numbers, remove this entire line if you don't want the numbers.
% 	aboveskip=0pt,belowskip=0pt,%
% 	showstringspaces=false,tabsize=2,breaklines=true}
% \floatstyle{ruled}
% \newfloat{listing}{tb}{lst}{}
% \floatname{listing}{Listing}

% \usepackage{booktabs}       
% \usepackage{adjustbox}
% \usepackage{multirow}
% \usepackage{siunitx}

% \usepackage{amsmath}
% \usepackage{amssymb}
% \usepackage{mathtools}
% \usepackage{amsthm}
% \usepackage{mathabx}
% \usepackage{array}
% \usepackage{rotating}

% \usepackage{enumitem}
% \usepackage{subfigure}
% \setlist[enumerate]{nosep}
% \usepackage{soul}
% \usepackage{caption}
% \usepackage{xcolor}
% \usepackage{xspace}
% \usepackage{arydshln}
% \usepackage{MnSymbol,pifont}


% % Dialect macros
% \newcommand{\IndEng}{en-IN\xspace}
% \newcommand{\USEng}{en-US\xspace}
% \newcommand{\Trans}{en-TR\xspace}
% \newcommand{\Multi}{en-MV\xspace}

% \newcommand{\gptf}{\textsc{gpt-4}\xspace}
% \newcommand{\llama}{\textsc{llama-3}\xspace}

% % Dataset macros
% \newcommand{\md}{MD3\xspace}
% \newcommand{\mmd}{M-MD3\xspace}

% \title{Evaluating Dialect Robustness of Language Models via Conversation Understanding}
% \date{\vspace{-5ex}Supplementary Material}

% \begin{document}
% \maketitle
% \section{Dataset Construction}\label{sec:masking}
% Table~\ref{tab:mask} describes the example conversations from extended \md and their corresponding masked versions from \mmd. We mask the turn where the guesser utters the target word to help with formulating our downstream tasks. We mask the target word by finding the exact match in the conversation as shown in the conversations from Table~\ref{tab:mask}. In case of conversations where an exact match is not found (such as \textit{planets}), we find the utterance that is most similar to the target word using the similarity score\footnote{Described in the \textit{Metrics} section of the main paper.}. The rest of the conversation is then pruned to make the masked target word (represented by `[MASK]') the last token in the conversation.

% % correction: fishermen to planet in the description

% \begin{table*}[h!]
%     \begin{adjustbox}{width=\linewidth,center}
%         \renewcommand{\arraystretch}{1}
%         \begin{tabular}{cp{18em}p{18em}}
%             \toprule
%             \multicolumn{1}{>{\centering\arraybackslash}m{4em}}{\textbf{Target Word}} & \multicolumn{1}{>{\centering\arraybackslash}m{18em}}{\textbf{\IndEng}} & \multicolumn{1}{>{\centering\arraybackslash}m{18em}}{\textbf{Masked \IndEng}} \\\midrule[\heavyrulewidth]
%             \multirow{4}{4em}{\centering Fisherman} & \texttt{{Describer:} Uh. What do you call if we, what will be there in the water?} & \texttt{{Describer:} Uh. What do you call if we, what will be there in the water?}\\
%             & \texttt{{Guesser:} Fishes} & \texttt{{Guesser:} Fishes}\\
%             & \texttt{{Describer:} Who will catch that?} & \texttt{{Describer:} Who will catch that?}\\
%             & \texttt{{Guesser:} \textit{\underline{\textbf{Fisherman}}}.} & \texttt{{Guesser:} \textit{\underline{\textbf{[MASK]}}}}\\\midrule[\heavyrulewidth]
%             \multicolumn{1}{>{\centering\arraybackslash}m{4em}}{\textbf{Target Word}} & \multicolumn{1}{>{\centering\arraybackslash}m{18em}}{\textbf{\USEng}} & \multicolumn{1}{>{\centering\arraybackslash}m{18em}}{\textbf{Masked \USEng}} \\\midrule[\heavyrulewidth]
%             \multirow{3}{4em}{\centering Planet} & \texttt{{Describer:} These are hard words. um Okay. So there's. the Sun and the Moon and all the rest of them.} & \texttt{{Describer:} These are hard words. um Okay. So there's. the Sun and the Moon and all the rest of them.}\\
%             & \texttt{Guesser: And all the \textit{\underline{\textbf{planet}}}s?} & \texttt{Guesser: \textit{\underline{\textbf{[MASK]}}}}\\
%             & \texttt{\textbf{(}Describer: Yes.\textbf{)}} & \\
%             \bottomrule
%         \end{tabular}
%     \end{adjustbox}
%     \caption{Masking conversations from the extended \md to create \mmd. The text such as \texttt{\textit{\textbf{\underline{this}}}} represents the target word utterance by the guesser which is masked (represented by, \texttt{\textit{\textbf{\underline{[MASK]}}}} in the \mmd version of the conversation. The rest of the original conversation is pruned as represented text in parentheses.}
%     \label{tab:mask}
% \end{table*}
% \section{Transformation Issues}
% % correct: into \Trans
% We transform conversations from \IndEng into \Trans, by prompting\footnote{The exact prompt can be found in the \textit{Methodology} section of the main paper.} \gptf to remove exaggerations and dialectal information. As mentioned in Table~\ref{tab:trans}, a \textit{`typical'} transformed conversation maintains the semantic meaning but only differs from the original conversation grammatically. A \textit{`bad'} example deviates largely from the expected output, and such examples are excluded from the final set of conversations used in our evaluation.
% \begin{table*}[h!] 
%     \begin{adjustbox}{width=\linewidth,center}
%         \renewcommand{\arraystretch}{1}
%         \begin{tabular}{cp{18em}p{18em}}
%             \toprule
%             \multicolumn{1}{>{\centering\arraybackslash}m{6em}}{\textbf{Type}} & \multicolumn{1}{>{\centering\arraybackslash}m{18em}}{\textbf{\IndEng}} & \multicolumn{1}{>{\centering\arraybackslash}m{18em}}{\textbf{\Trans}} \\\midrule[\heavyrulewidth]
%             \multirow{4}{6em}{\centering Typical}& \texttt{{Describer:} \textbf{(}Uh\textbf{)}. What do you call \textit{\underline{\textbf{if we, what will be there}}} in the water?} & \texttt{{Describer:} \textbf{(}$\varnothing$\textbf{)} What do you call \textit{\underline{\textbf{the creatures}}} in the water?}\\
%             & \texttt{{Guesser:} Fish\textbf{(}es\textbf{)}} & \texttt{{Guesser:} Fish\textbf{(}$\varnothing$\textbf{)}.}\\
%             & \texttt{{Describer:} Who \textit{\underline{\textbf{will catch that}}}?} & \texttt{{Describer:} Who \textit{\underline{\textbf{catches them}}}?}\\
%             & \texttt{{Guesser:} Fisherm\textit{\underline{\textbf{a}}}n.} & \texttt{{Guesser:} Fisherm\textit{\underline{\textbf{e}}}n.}\\\midrule[\heavyrulewidth]
%             \multirow{10}{6em}{\centering Bad}& \texttt{{Describer:} There. is a. there is a character in a movie} & \multirow{10}{18em}{The character being described is from a well-known movie and is known for the line ``I am still gorgeous.'' This character is similar to those found in Marvel movies and has a very muscular physique, which is achieved through scientific injections that cause his body to grow. The character being guessed is Captain America.}\\
%             & \texttt{{Guesser:} um} & \\
%             & \texttt{{Describer:} It's a very famous movie and it's a very. where is a where you can see famous dialogue called I am still gorgeous} & \\
%             & \texttt{{Guesser:} uh. ok. uh} & \\
%             & \texttt{{Describer:} character name. compare like Marvel movie} & \\
%             & \texttt{{Guesser:} So. uh} & \\
%             & \texttt{{Describer:} very muscular body gives scientifically. injections} &\\
%             & \texttt{{Guesser:} ok} & \\
%             & \texttt{{Describer:} His body will grow} & \\
%             & \texttt{{Guesser:} uh Captain America} & \\
%             \bottomrule
%         \end{tabular}
%     \end{adjustbox}
%     \caption{Example \textit{transformations} of \IndEng to \Trans. We utilise \gptf to generate the response. The text in parentheses refers to the omission/removal of certain filler and exaggerated words, and the text such as \texttt{\textit{\textbf{\underline{this}}}}, refers to the words or sentences that were rephrased to convey the original meaning.}
%     \label{tab:trans}
% \end{table*}

% \section{Errors}
% Table~\ref{tab:errors} describes additional examples for all identified error types\footnote{defined in the \textit{Error Analysis} section of the main paper.}. As mentioned, each conversation can be classified under multiple error types. For example, the conversation about the target word--\textit{`Ryan Reynolds'} is classified as \textbf{CC}, but can also be classified as \textbf{PF}.


% \begin{table*}[h!] 
%     \begin{adjustbox}{width=1\linewidth,center}
%         \renewcommand{\arraystretch}{1}
%         \begin{tabular}{ccp{35em}c}
%             \toprule
%             \multicolumn{1}{>{\centering\arraybackslash}m{2em}}{\textbf{Type}} & \multicolumn{1}{>{\centering\arraybackslash}m{6em}}{\textbf{Target Word}} & \multicolumn{1}{>{\centering\arraybackslash}m{18em}}{\textbf{Conversation}} & \multicolumn{1}{>{\centering\arraybackslash}m{6em}}{\textbf{Model Prediction}}\\\midrule[\heavyrulewidth]
%             \multirow{2}{2em}{\centering \textbf{AD}}& \multirow{2}{6em}{\centering Fisherman} & \texttt{{Describer:} Okay. Okay. A. guy um wants to um okay. Guy catching something in the water.} & \multirow{2}{2em}{\centering Fish}\\
%             & & \texttt{{Guesser:} [MASK]} & \\\midrule[\heavyrulewidth]
%             \multirow{6}{2em}{\centering \textbf{WD}}& \multirow{6}{6em}{\centering Atlantic Ocean} & \texttt{Describer: One of the. of the of world.} & \multirow{6}{6em}{\centering Kanyakumari}\\
%             & & \texttt{Guesser: Of the seventh wonder of the world. Taj mahal? Is it regarding sea?} & \\
%             & & \texttt{Describer: No no no the. Towards the bottom of India.} & \\
%             & & \texttt{Guesser: Is it regarding} & \\
%             & & \texttt{Describer: what we have?} & \\
%             & & \texttt{Guesser: [MASK]} & \\\midrule[\heavyrulewidth]
%             \multirow{10}{2em}{\centering \textbf{BDD}}& \multirow{10}{6em}{\centering Russian Language}& \texttt{Describer: Ok. Ah Largest continent in the world} & \multirow{10}{6em}{\centering Russian}\\
%             & &  \texttt{Guesser: Ok.} & \\
%             & &  \texttt{Describer: Ah like area wise. Which country?} & \\
%             & &  \texttt{Guesser: Largest. vast area. vast area? Russia but.} & \\
%             & &  \texttt{Describer: We need to add N over there at the end.} & \\
%             & &  \texttt{Guesser: Russian} & \\
%             & &  \texttt{Describer: We speak} & \\
%             & &  \texttt{Guesser: What they speak?} & \\
%             & &  \texttt{Describer: Yeah. Ok.} & \\
%             & &  \texttt{Guesser: [MASK]} & \\\midrule[\heavyrulewidth]
%             \multirow{10}{2em}{\centering \textbf{CC}}& \multirow{10}{6em}{\centering Ryan Reynolds} & \texttt{Describer: It is like. One of the. Pen name. which we used in school school days.} & \multirow{10}{6em}{\centering Flair}\\
%             & & \texttt{Guesser: Cello point pen. Fine Grip} & \\
%             & & \texttt{Describer: No no no} & \\
%             & & \texttt{Guesser: Reynolds} & \\
%             & & \texttt{Describer: Uh yeah yeah} & \\
%             & & \texttt{Guesser: This is a second word or first word.} & \\
%             & & \texttt{Describer: Yeah this is second word} & \\
%             & & \texttt{Guesser: First word is. Name} & \\
%             & & \texttt{Describer:Yeah name related to the same} & \\
%             & & \texttt{Guesser: [MASK]} & \\\midrule[\heavyrulewidth]
%             \multirow{6}{2em}{\centering \textbf{PF}}& \multirow{6}{6em}{\centering Steve Jobs} & \texttt{Describer: Ok. He is a famous person and he is a. a. for. what we call? . Um now it is a. Its. giving competition to Android. what we call?} & \multirow{6}{6em}{\centering Steve}\\
%             & & \texttt{Guesser: ok. so he is the fond ok sorry } & \\
%             & & \texttt{Describer: he is a founder of so and so company. Its a U. S. company} & \\
%             & & \texttt{Guesser: so it is giving competition to Android means Google ok.. So} & \\
%             & & \texttt{Describer: and he is the founder of that company} & \\
%             & & \texttt{Guesser: [MASK]} & \\\midrule[\heavyrulewidth]
%             \multirow{2}{2em}{\centering \textbf{ERR}}& \multirow{2}{6em}{\centering Podium} &  \texttt{Describer: Okay um. uh. well I isn't sure I'm not sure but uh letting are seeing. Well it's like preacher are churching. I am standing behind this. uh. in in used for speaker.} & \multirow{2}{6em}{\centering Pulpit}\\
%             & &  \texttt{Guesser: [MASK]} & \\
%             \bottomrule
%         \end{tabular}
%     \end{adjustbox}
%     \caption{Example conversations (\textit{`Conversation'}) for each error type (\textit{`Type'}) along with the reference target word (\textit{`Target Word'}) and the generated target word (\textit{`Model Prediction'}). All model predictions are generated using the pre-trained variants of \gptf and \llama.}
%     \label{tab:errors}
% \end{table*}

% % doubt: predictions from which config

% \end{document}
